# Supplementary material for: L-valley Electron Spin Dynamics in GaAs
Source: arXiv:1207.5978 source file (2012-07-25)
Supplement: Supplementary file 1 [file Supplementary_Information.pdf]

**Supplementary information to**

L-valley electron spin dynamics in GaAs

T. Zhang, P. Barate, C. T. Nguyen, A. Balocchi, T. Amand, P. Renucci, H. Carrere, B. Urbaszek and X. Marie

*We present here the method to determine the photogenerated initial electron spin polarization in GaAs L valleys. In section I the general formalism to calculate the spin polarization of the photogenerated carriers in a conduction band from a given valence band is developed. This result is applied in section II to the specific case of photoexcited electrons in L valley for circularly polarized light propagating along [001].*

## I. General formalism

Assuming the laser excitation is slowly varying, the density matrix evolution of the conduction/valence electrons evolution is given, within time-dependent second order perturbation theory formulated in interaction representation, by:

$$\left(\frac{d\hat{\rho}^I}{dt}\right) = -\frac{1}{\hbar^2}\int_0^{\infty}\left[\hat{H}^I_{e-ph}(t+\tau),\left[\hat{H}^I_{e-ph}(t),\hat{\rho}(0)\right]\right]d\tau \quad \text{(S1)}$$

where:

$$\hat{H}^I_{e-ph}(t) = e^{i\frac{\hat{H}_0}{\hbar}t}\hat{H}_{e-ph}(t)e^{-i\frac{\hat{H}_0}{\hbar}t} = e^{i\frac{\hat{H}_0}{\hbar}t}\frac{e}{m_0 c}\mathbf{A}(t).\mathbf{p}\,e^{-i\frac{\hat{H}_0}{\hbar}t} \quad \text{(S2)}$$

is the electron-photon time dependent Hamiltonian in the interaction representation, and

$$\hat{H}_0(t) = \sum_{\nu,\mathbf{k}} E_{\nu,\mathbf{k}}\left|\psi_{\nu,\mathbf{k}}\right\rangle\left\langle\psi_{\nu,\mathbf{k}}\right| \quad \text{(S3)}$$

is the unperturbed electron hamiltonian for electron Bloch states $\left|\psi_{\nu,\mathbf{k}}\right\rangle$ of band ν and wave vector **k** with eigen-energy $E_{\nu,\mathbf{k}} = \hbar\omega_{\nu,\mathbf{k}}$ (here the summation is restricted to the first Brillouin zone). Note that, in virtue of Kramers theorem, the bands are twice degenerated in energy, so that $\nu \in (\nu_+, \nu_-)$. The vector potential is $\mathbf{A}\ (t) = \mathbf{A}_- e^{i(\mathbf{q}.\mathbf{r}-\omega t)} + \mathbf{A}_+ e^{-i(\mathbf{q}.\mathbf{r}-\omega t)}$ with $\omega = \frac{c}{n}|\mathbf{q}|$, **q** and $\mathbf{A}_+ = \mathbf{A}_-^*$ characterise the pulsation, wavevector and polarization of the single optical mode considered at this stage. For a stationary optical excitation, we can always define:

$$\hat{H}_{e-ph}(t) \equiv \hat{H}_+(t) + \hat{H}_-(t) \quad \text{(S4)}$$

Where, taking the Coulomb gauge: $\hat{H}_\pm(t) = \left(\hat{H}_\mp\right)^\dagger(t) \propto e^{\pm i\omega t}$. In the secular – and short correlation – approximations, (S1) can be evaluated by:

$$\left(\frac{d\hat{\rho}^I}{dt}\right) \approx -\frac{1}{\hbar^2}\int_0^{\infty}\left[\hat{H}_+(t+\tau),\left[\hat{H}_-(t),\hat{\rho}(0)\right]\right]d\tau + h.c. \quad \text{(S5)}$$

$$\left(\frac{d\hat{\rho}^I}{dt}\right) \approx \frac{1}{\hbar^2}\int_0^\infty \left[-\hat{H}_+(t+\tau)\hat{H}_-(t)\hat{\rho}(0) + \hat{H}_+(t+\tau)\hat{\rho}(0)\hat{H}_-(t) + \hat{H}_-(t)\hat{\rho}(0)\hat{H}_+(t+\tau) - \rho(0)\hat{H}_+(t+\tau)\hat{H}_-(t)\right] d\tau + h.c. \tag{S5bis}$$

where at $t = 0$, the initial electron density matrix is given at temperature T = 0 by:

$$\hat{\rho}(0) = \frac{1}{tr(\hat{\rho}(0))} \sum_{\substack{\mathbf{k} \\ \text{v}\in\{valencebands\}}} |\psi_{\nu,\mathbf{k}}\rangle\langle\psi_{\nu,\mathbf{k}}| = \frac{1}{2n_{val}N} \sum_{\substack{\mathbf{k} \\ \text{v}\in\{v.b.\}}} |u_{\nu,\mathbf{k}}\rangle\langle u_{\nu,\mathbf{k}}| \tag{S6}$$

Here, $N = V/\Omega$ is the number of crystal unit cells, $V$ and $\Omega$ are the volumes of the crystal and its unit cell respectively, and $2n_{val}$ is the total number of valence bands (the factor 2 stands for their degeneracy) and v $\in$ (v$_+$, v$_-$). Note this expression is still approximately valid when $k_B T << E_g$ . Due to Bloch theorem, we can write the electron states as: $|\psi_{\nu,\mathbf{k}}\rangle = \frac{1}{\sqrt{V}} e^{ik.r} |u_{\nu,\mathbf{k}}\rangle$, where $u_{\nu,\mathbf{k}}(\mathbf{r}) = \langle \mathbf{r}|u_{\nu,\mathbf{k}}\rangle$ is the periodic part of the Bloch function. We can then evaluate $\hat{H}_\pm(t)$ for interband transitions. For instance:

$$\hat{H}_-(t) = \frac{e}{m_0 c} e^{-i\omega t} \sum_{\nu,\nu',\mathbf{k}} \langle u_{\nu',\mathbf{k}+\mathbf{q}}|\mathbf{A}_-.\hat{\mathbf{p}}|u_{\nu,\mathbf{k}}\rangle |\psi_{\nu',\mathbf{k}+\mathbf{q}}\rangle\langle\psi_{\nu,\mathbf{k}}| \tag{S6}$$

so that:

$$\hat{H}_-^I(t) = \frac{e}{m_0 c} \sum_{\nu,\nu',\mathbf{k}} e^{-i(\omega - \omega_{\nu',\mathbf{k}+\mathbf{q}} + \omega_{\nu,\mathbf{k}})t} \langle u_{\nu',\mathbf{k}+\mathbf{q}}|\mathbf{A}_-.\hat{\mathbf{p}}|u_{\nu,\mathbf{k}}\rangle |\psi_{\nu',\mathbf{k}+\mathbf{q}}\rangle\langle\psi_{\nu,\mathbf{k}}| \tag{S7}$$

$$\hat{H}_+^I(t) = \left(\hat{H}_-^I(t)\right)^\dagger$$

We calculate here the contribution of the second and third term of (S5bis) to the evolution of the density matrix:

$$\left(\frac{d\hat{\rho}^I}{dt}\right)_+ = \frac{1}{n_\nu N}\left(\frac{e}{\hbar m_0 c}\right)^2 \Bigg\{ \int_{-\infty}^{\infty} d\tau$$

$$\sum_{\nu',\nu_1,\mathbf{k}'} e^{i(\omega - \omega_{\nu'_1,\mathbf{k}+\mathbf{q}} + \omega_{\nu,\mathbf{k}})\tau} \langle u_{\nu',\mathbf{k}'}|\mathbf{A}_+.\hat{\mathbf{p}}|u_{\nu_1,\mathbf{k}'+\mathbf{q}}\rangle |\psi_{\nu',\mathbf{k}'}\rangle\langle\psi_{\nu_1,\mathbf{k}'+\mathbf{q}}| \sum_{\text{v}\in\{v.b.\},\mathbf{k}''} |\psi_{\text{v},\mathbf{k}''}\rangle\langle\psi_{\text{v},\mathbf{k}''}| \sum_{\nu'_1,\nu,\mathbf{k}} \langle u_{\nu'_1,\mathbf{k}+\mathbf{q}}|\mathbf{A}_-.\hat{\mathbf{p}}|u_{\nu,\mathbf{k}}\rangle |\psi_{\nu'_1,\mathbf{k}+\mathbf{q}}\rangle\langle\psi_{\nu,\mathbf{k}}|$$

$$+$$

$$\sum_{\nu',\nu_1,\mathbf{k}'} e^{-i(\omega - \omega_{\nu'_1,\mathbf{k}+\mathbf{q}} + \omega_{\nu,\mathbf{k}})\tau} \langle u_{\nu',\mathbf{k}'+\mathbf{q}}|\mathbf{A}_-.\hat{\mathbf{p}}|u_{\nu_1,\mathbf{k}'}\rangle |\psi_{\nu',\mathbf{k}'}\rangle\langle\psi_{\nu_1,\mathbf{k}'+\mathbf{q}}| \sum_{\text{v}\in\{v.b.\},\mathbf{k}''} |\psi_{\text{v},\mathbf{k}''}\rangle\langle\psi_{\text{v},\mathbf{k}''}| \sum_{\nu'_1,\nu,\mathbf{k}} \langle u_{\nu'_1,\mathbf{k}}|\mathbf{A}_+.\hat{\mathbf{p}}|u_{\nu,\mathbf{k}+\mathbf{q}}\rangle |\psi_{\nu'_1,\mathbf{k}+\mathbf{q}}\rangle\langle\psi_{\nu,\mathbf{k}}| \Bigg\}$$

We then obtain after some manipulations :

$$\left(\frac{d\hat{\rho}^I}{dt}\right)_+ = \frac{1}{2n_{val}N}\left(\frac{e}{\hbar m_0 c}\right)^2 \Bigg\{$$

$$\sum_{\substack{\nu,\nu',\mathbf{k}\\ \mathrm{v}\in\{v.b.\}}} \int_{-\infty}^{+\infty} d\tau\, e^{i(\omega-\omega_{\mathrm{v},\mathbf{k+q}}+\omega_{\nu,\mathbf{k}})\tau} \langle u_{\nu',\mathbf{k}} | \mathbf{A}_{+}.\hat{\mathbf{p}} | u_{\mathrm{v},\mathbf{k+q}} \rangle \langle u_{\mathrm{v},\mathbf{k+q}} | \mathbf{A}_{-}.\hat{\mathbf{p}} | u_{\nu,\mathbf{k}} \rangle |\psi_{\nu',\mathbf{k}}\rangle\langle\psi_{\nu,\mathbf{k}}|$$

$$+ \sum_{\substack{\nu,\nu',\mathbf{k}\\ \mathrm{v}\in\{v.b.\}}} \int_{-\infty}^{+\infty} d\tau\, e^{-i(\omega-\omega_{\mathrm{v},\mathbf{k+q}}+\omega_{\nu,\mathbf{k}})\tau} \langle u_{\nu',\mathbf{k+q}} | \mathbf{A}_{-}.\hat{\mathbf{p}} | u_{\mathrm{v},\mathbf{k}} \rangle \langle u_{\mathrm{v},\mathbf{k}} | \mathbf{A}_{+}.\hat{\mathbf{p}} | u_{\nu,\mathbf{k+q}} \rangle |\psi_{\nu',\mathbf{k}}\rangle\langle\psi_{\nu,\mathbf{k}}| \ \Big\}$$

$$= \frac{2\pi}{2n_{val}N}\left(\frac{e}{\hbar m_0 c}\right)^2 \Big\{ \sum_{\substack{\nu,\nu',\mathbf{k}\\ \mathrm{v}\in\{v.b.\}}} \delta(\omega-\omega_{\mathrm{v},\mathbf{k+q}}+\omega_{\nu,\mathbf{k}}) \langle u_{\nu',\mathbf{k}} | \mathbf{A}_{+}.\hat{\mathbf{p}} | u_{\mathrm{v},\mathbf{k+q}} \rangle \langle u_{\mathrm{v},\mathbf{k+q}} | \mathbf{A}_{-}.\hat{\mathbf{p}} | u_{\nu,\mathbf{k}} \rangle |\psi_{\nu',\mathbf{k}}\rangle\langle\psi_{\nu,\mathbf{k}}|$$

$$+ \sum_{\substack{\nu,\nu',\mathbf{k}\\ \mathrm{v}\in\{v.b.\}}} \delta(\omega-\omega_{\mathrm{v},\mathbf{k+q}}+\omega_{\nu,\mathbf{k}}) \langle u_{\nu',\mathbf{k+q}} | \mathbf{A}_{-}.\hat{\mathbf{p}} | u_{\mathrm{v},\mathbf{k}} \rangle \langle u_{\mathrm{v},\mathbf{k}} | \mathbf{A}_{+}.\hat{\mathbf{p}} | u_{\nu,\mathbf{k+q}} \rangle |\psi_{\nu',\mathbf{k}}\rangle\langle\psi_{\nu,\mathbf{k}}| \ \Big\}$$

$$\left(\frac{d\hat{\rho}^I}{dt}\right)_{+} = \frac{2\pi}{2n_{val}N}\left(\frac{e}{\hbar m_0 c}\right)^2 \sum_{\substack{\nu,\nu',\mathbf{k}\\ \mathrm{v}\in\{v.b.\}}} \delta(\omega-\omega_{\mathrm{v},\mathbf{k+q}}+\omega_{\nu,\mathbf{k}})$$

$$\times\Big[\langle u_{\nu',\mathbf{k}} | \mathbf{A}_{+}.\hat{\mathbf{p}} | u_{\mathrm{v},\mathbf{k+q}} \rangle \langle u_{\mathrm{v},\mathbf{k+q}} | \mathbf{A}_{-}.\hat{\mathbf{p}} | u_{\nu,\mathbf{k}} \rangle + \left(\langle u_{\nu,\mathbf{k+q}} | \mathbf{A}_{+}.\hat{\mathbf{p}} | u_{\mathrm{v},\mathbf{k}} \rangle \langle u_{\mathrm{v},\mathbf{k}} | \mathbf{A}_{-}.\hat{\mathbf{p}} | u_{\nu',\mathbf{k+q}} \rangle\right)^{*}\Big] |\psi_{\nu',\mathbf{k}}\rangle\langle\psi_{\nu,\mathbf{k}}| \qquad \text{(S8)}$$

The calculation can be done for the $\left(\frac{d\hat{\rho}^I}{dt}\right)_{-}$ contribution, but as we shall see, will not be useful in the frame of the low depletion approximation of the valence bands, and the form of the matrix elements close to Γ and L points.

For transitions close to a high symmetry point in the Brillouin zone like Γ, L, X corresponding to some energy bands extrema, since |**q**|<<π/a, (the typical Brillouin zone dimension in **k**-space) we can make the approximation $|u_{\nu,\mathbf{k}}\rangle \approx |u_{\nu,\mathbf{k}_0}\rangle$ with $\mathbf{k}_0 = \{\mathbf{k}_L, \mathbf{k}_\Gamma, \mathbf{k}_X\}$, which allows us to use the **k.p** approach to describe band states. The density matrix generation term (S8) can thus be approximated, as soon as |**k**|>>|**q**|, by :

$$\left(\frac{d\hat{\rho}^I}{dt}\right)_{+} = \frac{2\pi}{2n_{val}N}\left(\frac{e}{\hbar m_0 c}\right)^2 \Big[\langle u_{\nu',\mathbf{k}_0} | \mathbf{A}_{+}.\hat{\mathbf{p}} | u_{\mathrm{v},\mathbf{k}_0} \rangle \langle u_{\mathrm{v},\mathbf{k}_0} | \mathbf{A}_{-}.\hat{\mathbf{p}} | u_{\nu,\mathbf{k}_0} \rangle + \left(\langle u_{\nu,\mathbf{k}_0} | \mathbf{A}_{+}.\hat{\mathbf{p}} | u_{\mathrm{v},\mathbf{k}_0} \rangle \langle u_{\mathrm{v},\mathbf{k}_0} | \mathbf{A}_{-}.\hat{\mathbf{p}} | u_{\nu',\mathbf{k}_0} \rangle\right)^{*}\Big]\times$$

$$\times \sum_{\substack{\nu,\nu'\\ \mathrm{v}\in\{v.b.\}}} \Big[\langle u_{\nu',\mathbf{k}_0} | \mathbf{A}_{+}.\hat{\mathbf{p}} | u_{\mathrm{v},\mathbf{k}_0} \rangle \langle u_{\mathrm{v},\mathbf{k}_0} | \mathbf{A}_{-}.\hat{\mathbf{p}} | u_{\nu,\mathbf{k}_0} \rangle + \left(\langle u_{\nu,\mathbf{k}_0} | \mathbf{A}_{+}.\hat{\mathbf{p}} | u_{\mathrm{v},\mathbf{k}_0} \rangle \langle u_{\mathrm{v},\mathbf{k}_0} | \mathbf{A}_{-}.\hat{\mathbf{p}} | u_{\nu',\mathbf{k}_0} \rangle\right)^{*}\Big]\times$$

$$\times \sum_{\mathbf{k}} \delta(\omega-\omega_{\mathrm{v},\mathbf{k}}+\omega_{\nu,\mathbf{k}}) \times |\psi_{\nu',\mathbf{k}}\rangle\langle\psi_{\nu,\mathbf{k}}| \qquad \text{(S9)}$$

Since : $\sum_{\mathbf{k}} \delta(\omega-\omega_{\mathrm{v},\mathbf{k}}+\omega_{\nu,\mathbf{k}}) \times |\psi_{\nu',\mathbf{k}}\rangle\langle\psi_{\nu,\mathbf{k}}| = \hbar\frac{V}{(2\pi)^3}\int d^3\mathbf{k}\ \delta\left(E-E_{\mathrm{v},\nu}(\mathbf{k})\right)|\psi_{\nu',\mathbf{k}}\rangle\langle\psi_{\nu,\mathbf{k}}|$

we obtain :

$$\left(\frac{d\hat{\rho}^I}{dt}\right)_{+} = \frac{2\pi}{\hbar}\frac{1}{2n_{val}N}\left(\frac{e}{m_0 c}\right)^2$$

$$\times \sum_{\substack{\nu,\nu' \\ \mathrm{v}\in\{v.b.\}}} \left[ \langle u_{\nu',\mathbf{k}_0} | \mathbf{A}_+ .\hat{\mathbf{p}} | u_{\mathrm{v},\mathbf{k}_0} \rangle \langle u_{\mathrm{v},\mathbf{k}_0} | \mathbf{A}_- .\hat{\mathbf{p}} | u_{\nu,\mathbf{k}_0} \rangle + \left( \langle u_{\nu,\mathbf{k}_0} | \mathbf{A}_+ .\hat{\mathbf{p}} | u_{\mathrm{v},\mathbf{k}_0} \rangle \langle u_{\mathrm{v},\mathbf{k}_0} | \mathbf{A}_- .\hat{\mathbf{p}} | u_{\nu',\mathbf{k}_0} \rangle \right)^* \right] \times$$

$$\times \sum_{\mathbf{k}} \delta(E - E_{\mathrm{v},\mathbf{k}} + E_{\nu,\mathbf{k}}) \times |\psi_{\nu',\mathbf{k}}\rangle\langle\psi_{\nu,\mathbf{k}}| \quad \text{(S10)}$$

Let : $E_{\mathrm{v},\nu}(\mathbf{k}) \equiv E_{\mathrm{v}}(\mathbf{k}) - E_\nu(\mathbf{k})$, so that $\delta E_{\mathrm{v},\nu}(\mathbf{k}) = \nabla_{\mathbf{k}}(E_{\mathrm{v},\nu}(\mathbf{k})).\delta\mathbf{k} = |\nabla_{\mathbf{k}}(E_{\mathrm{v},\nu}(\mathbf{k}))|\, dk_\| \, d^2\mathbf{k}_\perp$.

$$\sum_{\mathbf{k}} \delta(E - E_{\mathrm{v},\mathbf{k}} + E_{\nu,\mathbf{k}}) \times |\psi_{\nu',\mathbf{k}}\rangle\langle\psi_{\nu,\mathbf{k}}| = \frac{V}{(2\pi)^3} \int \frac{\delta(E - E_{\mathrm{v},\nu})}{|\nabla_{\mathbf{k}}(E_{\mathrm{v},\nu}(\mathbf{k}))|} dE_{\mathrm{v},\nu} \int d^2\mathbf{k}_\perp |\psi_{\nu',\mathbf{k}}\rangle\langle\psi_{\nu,\mathbf{k}}|$$

$$= \frac{1}{(2\pi)^3} \frac{1}{|\nabla_{\mathbf{k}}(E_{\mathrm{v},\nu}(\mathbf{k}))|_{E_{\mathrm{v},\nu}(\mathbf{k})=E}} \int_{\mathsf{S}_{\mathrm{v},\nu}(E)} d^2\mathbf{k}_\perp |u_{\nu',k_0}\rangle\langle u_{\nu,k_0}|$$

$$= \frac{1}{(2\pi)^3} \frac{\mathsf{S}_{\mathrm{v},\nu}(E)}{|\nabla_{\mathbf{k}}(E_{\mathrm{v},\nu}(\mathbf{k}))|_{E_{\mathrm{v},\nu}(\mathbf{k})=E}} |u_{\nu',k_0}\rangle\langle u_{\nu,k_0}|$$

We introduce the energy joint density of states $\mathsf{D}_{\nu',\nu}(E)$ for a transition from band ν to ν′ :

$$\mathsf{D}_{\nu',\nu}(E) = \frac{V}{(2\pi)^3} \frac{\mathsf{S}_{\mathrm{v},\nu}(E)}{|\nabla_{\mathbf{k}}(E_{\mathrm{v},\nu}(\mathbf{k}))|_{E_{\mathrm{v},\nu}(\mathbf{k})=E}} \quad \text{(S11)}$$

where $\mathsf{S}_{\mathrm{v},\nu}(E)$ is the surface in **k**-space where the equation $E_{\mathrm{v},\nu}(\mathbf{k}) = E$ is satisfied.

$$\sum_{\mathbf{k}} \delta(E - E_{\mathrm{v},\mathbf{k}} + E_{\nu,\mathbf{k}}) \times |\psi_{\nu',\mathbf{k}}\rangle\langle\psi_{\nu,\mathbf{k}}| = \mathsf{D}_{\nu',\nu}(E) |u_{\nu',k_0}\rangle\langle u_{\nu,k_0}|$$

Finally, we obtain :

$$\left(\frac{d\hat{\rho}^I}{dt}\right)_+ = \frac{2\pi}{\hbar} \frac{1}{2n_{val}N} \left(\frac{e}{m_0 c}\right)^2 \times$$

$$\times \sum_{\substack{\nu,\nu' \\ \mathrm{v}\in\{v.b.\}}} \left[ \langle u_{\nu',\mathbf{k}_0} | \mathbf{A}_+ .\hat{\mathbf{p}} | u_{\mathrm{v},\mathbf{k}_0} \rangle \langle u_{\mathrm{v},\mathbf{k}_0} | \mathbf{A}_- .\hat{\mathbf{p}} | u_{\nu,\mathbf{k}_0} \rangle + \left( \langle u_{\nu,\mathbf{k}_0} | \mathbf{A}_+ .\hat{\mathbf{p}} | u_{\mathrm{v},\mathbf{k}_0} \rangle \langle u_{\mathrm{v},\mathbf{k}_0} | \mathbf{A}_- .\hat{\mathbf{p}} | u_{\nu',\mathbf{k}_0} \rangle \right)^* \right] \times$$

$$\times \frac{V}{(2\pi)^3} \frac{1}{|\nabla_{\mathbf{k}}(E_{\mathrm{v},\nu}(\mathbf{k}))|_{E_{\mathrm{v},\nu}(\mathbf{k})=E}} \int_{\mathsf{S}_{\nu',\nu}(E)} d^2\mathbf{k}_\perp |\psi_{\nu'}(\mathbf{k})\rangle\langle\psi_\nu(\mathbf{k})|$$

The population generation rate in a given conduction band $c_j$ ($j = \pm$) writes then:

$$\frac{dN_{c_j}}{dt} = tr_\nu \left(\frac{d\hat{\rho}^I}{dt}\right)_+ ,$$

so that: $$\frac{dN_{c_j}}{dt}=\frac{2\pi}{\hbar}\left(\frac{eA_0}{m_0c}\right)^2\frac{1}{2n_{val}}\sum_{v}^{n_{val}}\mathsf{D}_{v,c}(E)\sum_{i=+,-}\left|\left\langle u_{c_j,\mathbf{k}_0}\left|\mathbf{e}_\pm.\hat{\mathbf{p}}\right|u_{v_i,\mathbf{k}_0}\right\rangle\right|^2 \qquad \text{(S12)}$$

where $A_0\equiv\left|\mathbf{A}_\pm\right|$ and $\mathbf{e}_\pm\equiv\mathbf{A}_\pm/A_0$. Note that since $tr\left(\hat{\rho}^I\right)=1$, the population generation rate in a conduction band is exactly compensated by the population decay rate in the valence bands, which is estimated from $\left(\frac{d\hat{\rho}^I}{dt}\right)_-$. The total population generated in the conduction band is :

$$\frac{dN_c}{dt}=\frac{dN_{c_+}}{dt}+\frac{dN_{c_-}}{dt}$$

The total electron spin generation rate $\frac{d\mathbf{S}_c}{dt}$ in a given conduction band c. It writes:

$$\frac{d\mathbf{S}_c}{dt}=\frac{d\left\langle\hat{\mathbf{S}}_c\right\rangle}{dt}=tr_c\left[\left(\frac{d\hat{\rho}^I}{dt}\right)_+\hat{\mathbf{S}}\right]$$

where $\hat{\mathbf{S}}=\frac{\hbar}{2}\left(\hat{\sigma}_x,\hat{\sigma}_y,\hat{\sigma}_z\right)$, and $\left(\hat{\sigma}_x,\hat{\sigma}_y,\hat{\sigma}_z\right)$ are the Pauli matrixes. For the $S_{c,z}$ component for instance, we obtain from (S10) :

$$\left(\frac{dS_{c,z}}{dt}\right)_+=\frac{2\pi}{\hbar}\frac{1}{n_{val}N}\left(\frac{e}{m_0c}\right)^2\times$$

$$\times tr_c\Bigg(\sum_{\substack{c,c'\\ v\in\{v.b.\}}}\left[\left\langle u_{c',\mathbf{k}_0}\left|\mathbf{A}_+.\hat{\mathbf{p}}\right|u_{v,\mathbf{k}_0}\right\rangle\left\langle u_{v,\mathbf{k}_0}\left|\mathbf{A}_-.\hat{\mathbf{p}}\right|u_{c,\mathbf{k}_0}\right\rangle+\left(\left\langle u_{c,\mathbf{k}_0}\left|\mathbf{A}_+.\hat{\mathbf{p}}\right|u_{v,\mathbf{k}_0}\right\rangle\left\langle u_{v,\mathbf{k}_0}\left|\mathbf{A}_-.\hat{\mathbf{p}}\right|u_{c',\mathbf{k}_0}\right\rangle\right)^*\right]\times$$
$$\times\sum_{\mathbf{k}}\delta(E-E_{v,\mathbf{k}}+E_{c,\mathbf{k}})\left|\psi_{c',\mathbf{k}}\right\rangle\left\langle\psi_{c,\mathbf{k}}\right|\hat{S}_z\Bigg)$$

$$=\frac{2\pi}{\hbar}\frac{1}{n_{val}N}\left(\frac{e}{m_0c}\right)^2\times$$

$$\times tr_c\Bigg(\sum_{\substack{c\\ v\in\{v.b.\}}}\left[\left\langle u_{c,\mathbf{k}_0}\left|\mathbf{A}_+.\hat{\mathbf{p}}\right|u_{v,\mathbf{k}_0}\right\rangle\left\langle u_{v,\mathbf{k}_0}\left|\mathbf{A}_-.\hat{\mathbf{p}}\right|u_{c,\mathbf{k}_0}\right\rangle+\left(\left\langle u_{c,\mathbf{k}_0}\left|\mathbf{A}_+.\hat{\mathbf{p}}\right|u_{v,\mathbf{k}_0}\right\rangle\left\langle u_{v,\mathbf{k}_0}\left|\mathbf{A}_-.\hat{\mathbf{p}}\right|u_{c,\mathbf{k}_0}\right\rangle\right)^*\right]\times$$
$$\times\sum_{\mathbf{k}}\delta(E-E_{v,\mathbf{k}}+E_{c,\mathbf{k}})\left|\psi_{c,\mathbf{k}}\right\rangle\left\langle\psi_{c,\mathbf{k}}\right|\hat{S}_z\Bigg)$$

$$\left(\frac{dS_{c,z}}{dt}\right)_+=\frac{2\pi}{\hbar}\frac{1}{n_{val}N}\left(\frac{e}{m_0c}\right)^2\sum_{\substack{i=+,-\\ v\in\{v.b.\}}}\frac{\hbar}{2}\left[\left|\left\langle u_{v_i,\mathbf{k}_0}\left|\mathbf{e}_-.\hat{\mathbf{p}}\right|u_{c_+,\mathbf{k}_0}\right\rangle\right|^2-\left|\left\langle u_{v_i,\mathbf{k}_0}\left|\mathbf{e}_+.\hat{\mathbf{p}}\right|u_{c_-,\mathbf{k}_0}\right\rangle\right|^2\right]\sum_{\mathbf{k}}\delta(E-E_{v,\mathbf{k}}+E_{c,\mathbf{k}}) \qquad \text{(S13)}$$

we obtain finally :

$$\left(\frac{dS_{c,z}}{dt}\right)_+ = \frac{2\pi}{\hbar}\frac{1}{n_{val}N}\left(\frac{e}{m_0 c}\right)^2 \sum_{\substack{i=+,-\\ v\in\{v.b.\}}} \frac{\hbar}{2}\left[\left|\left\langle u_{v_i,\mathbf{k}_0}\right|\mathbf{e}_-.\hat{\mathbf{p}}\left|u_{c_+,\mathbf{k}_0}\right\rangle\right|^2 - \left|\left\langle u_{v_i,\mathbf{k}_0}\right|\mathbf{e}_+.\hat{\mathbf{p}}\left|u_{c_-,\mathbf{k}_0}\right\rangle\right|^2\right]\sum_{\mathbf{k}}\delta(E-E_{v,\mathbf{k}}+E_{c,\mathbf{k}})$$

$$\left(\frac{dS_{c,z}}{dt}\right)_+ = \frac{2\pi}{\hbar}\frac{1}{n_{val}N}\left(\frac{e}{m_0 c}\right)^2 \mathrm{D}_{v,c}(E) \sum_{\substack{i=+,-\\ v\in\{v.b.\}}} \frac{\hbar}{2}\left[\left|\left\langle u_{v_i,\mathbf{k}_0}\right|\mathbf{e}_-.\hat{\mathbf{p}}\left|u_{c_+,\mathbf{k}_0}\right\rangle\right|^2 - \left|\left\langle u_{v_i,\mathbf{k}_0}\right|\mathbf{e}_+.\hat{\mathbf{p}}\left|u_{c_-,\mathbf{k}_0}\right\rangle\right|^2\right] \tag{S14}$$

and, from (S12) and (S14), the spin polarization of the generated carriers in a conduction band from a given valence band is simply:

$$S_{c,z}\Big|_{gen} = \frac{\hbar}{2}\frac{\left[\left|\left\langle u_{v_i,\mathbf{k}_0}\right|\mathbf{e}_-.\hat{\mathbf{p}}\left|u_{c_+,\mathbf{k}_0}\right\rangle\right|^2 - \left|\left\langle u_{v_i,\mathbf{k}_0}\right|\mathbf{e}_+.\hat{\mathbf{p}}\left|u_{c_-,\mathbf{k}_0}\right\rangle\right|^2\right]}{\left|\left\langle u_{c_j,\mathbf{k}_0}\right|\mathbf{e}_-.\hat{\mathbf{p}}\left|u_{v_i,\mathbf{k}_0}\right\rangle\right|^2 + \left|\left\langle u_{c_j,\mathbf{k}_0}\right|\mathbf{e}_+.\hat{\mathbf{p}}\left|u_{v_i,\mathbf{k}_0}\right\rangle\right|^2} \tag{S15}$$

The calculation of $S_{c,x}\Big|_{gen}$ and $S_{c,y}\Big|_{gen}$ can be performed with the same method.

Finally, it is also possible to extend this formalism to slowly varying laser pulses by replacing $A_0$ by a slowly varying function of time $A_0(t)$, *i.e.* pulses with duration much longer than the correlation time of electronic states (which is typically the case with laser pulses of ~1 ps duration used here).

## II. Calculation of the photogenerated electron spin polarization in L valleys.

We turn now to the specific problem of optical pumping of spin oriented electrons in the GaAs L-valleys. Here, the excitation is provided by a laser beam assumed to propagate along the [001] direction with $\sigma^+$ polarisation.

Lets us define the laboratory frame $\mathcal{B}$ = {$\mathbf{e}_x$, $\mathbf{e}_y$, $\mathbf{e}_z$} with unit vectors oriented respectively along the [100], [010] and [001] crystallographic directions. To deal with circularly polarised light, it is convenient to introduce the spinorial basis [1] as $\mathcal{B}_S$ = {$\mathbf{e}_+$, $\mathbf{e}_-$, $\mathbf{e}_0$} with:

$$\mathbf{e}_+ = -\frac{1}{\sqrt{2}}(\mathbf{e}_x + i\mathbf{e}_y),\ \mathbf{e}_- = \frac{1}{\sqrt{2}}(\mathbf{e}_x - i\mathbf{e}_y),\ \mathbf{e}_0 = \mathbf{e}_z \tag{S16}$$

The spinorial components of any vector $\mathbf{A}$ are, in this complex orthonormal basis write :

$$A_+ = -\frac{1}{\sqrt{2}}(A_x - iA_y),\ A_- = \frac{1}{\sqrt{2}}(A_x + iA_y),\ \ A_0 = A_z$$

Note that with these definitions: $\mathbf{e}_\mp = -\mathbf{e}_\mp^*$, and $A_\mp = -A_\mp^*$. Taking

$$\mathbf{A}(\mathbf{r},t) = A_0\left[\cos(\omega t - \mathbf{q}.\mathbf{r})\mathbf{e}_x + \sin(\omega t - \mathbf{q}.\mathbf{r})\mathbf{e}_y\right]$$

as the vector potential of a $\sigma^+$ polarised laser beam propagating along the [001] direction with, its expression in $\mathcal{B}_S$ frame is:

$$\mathbf{A}(\mathbf{r},t)=\frac{A_0}{\sqrt{2}}\left[-e^{i(\mathbf{q}.\mathbf{r}-\omega t)}\mathbf{e}_+ + e^{-i(\mathbf{q}.\mathbf{r}-\omega t)}\mathbf{e}_-\right]$$

This description, suitable for optical transitions close to Γ point where the symmetry of the crystal is $T_d$ , is not convenient for the transitions close to the L point. As a fact, the local symmetry at $\mathbf{k}_L$ point is $C_{3v}$ [2], with the quantification axis z' along a <111> direction, and the electronic states symmetry and the coupling tables by operators can be deduced simply within this new frame. We are thus led to define a new basis $\mathcal{B}'$. Among the 8 different possible choices for the $L_i$ ($i$=1,…,8) valleys, we select the one oriented along [111], labelled $L_1$ , and define the corresponding frame as :

$$\mathbf{e}_{x'}=\frac{1}{\sqrt{6}}(\mathbf{e}_x+\mathbf{e}_y-2\mathbf{e}_z),\ \mathbf{e}_{y'}=\frac{1}{\sqrt{6}}(\mathbf{e}_x-\mathbf{e}_y),\ \mathbf{e}_{z'}=\frac{1}{\sqrt{6}}(\mathbf{e}_x+\mathbf{e}_y+\mathbf{e}_z)$$

The corresponding spinorial basis is $\mathcal{B}'_S$ defined by:

$$\mathbf{e}'_+=-\frac{1}{\sqrt{2}}(\mathbf{e}'_x+i\mathbf{e}'_y),\ \mathbf{e}'_-=\frac{1}{\sqrt{2}}(\mathbf{e}'_x-i\mathbf{e}'_y),\ \mathbf{e}'_0=\mathbf{e}'_z \qquad \text{(S16)}$$

The passage matrix from the basis $\mathcal{B}_S$ to the basis $\mathcal{B}'_S$ can be thoroughly deduced as :

$$[P]_{\mathcal{B}_S,\mathcal{B}'_S}=\begin{bmatrix} -\frac{e^{i\frac{\pi}{4}}}{2}\left(1+\frac{1}{\sqrt{3}}\right) & -\frac{e^{i\frac{\pi}{4}}}{2}\left(1-\frac{1}{\sqrt{3}}\right) & \frac{e^{i\frac{\pi}{4}}}{\sqrt{3}} \\ -\frac{e^{-i\frac{\pi}{4}}}{2}\left(1-\frac{1}{\sqrt{3}}\right) & -\frac{e^{-i\frac{\pi}{4}}}{2}\left(1+\frac{1}{\sqrt{3}}\right) & -\frac{e^{-i\frac{\pi}{4}}}{\sqrt{3}} \\ \frac{1}{\sqrt{3}} & \frac{1}{\sqrt{3}} & \frac{1}{\sqrt{3}} \end{bmatrix} \qquad \text{(S17)}$$

Which is unitary, since the two complex basis are orthonormal. The spinorial components of any vector $[\mathbf{r}]_{\mathcal{B}_S}=[r_+,r_-,r_0]$, $[\mathbf{r}]_{\mathcal{B}'_S}=[r'_+,r'_-,r'_0]$transform as : $[\mathbf{r}]_{\mathcal{B}_S}=[P]_{\mathcal{B}_S,\mathcal{B}'_S}[\mathbf{r}]_{\mathcal{B}'_S}$ , so that : $[\mathbf{r}]_{\mathcal{B}'_S}=[P]^{\dagger}_{\mathcal{B}_S,\mathcal{B}'_S}[\mathbf{r}]_{\mathcal{B}_S}$ . Note that these transformation laws apply to any vectorial operator as well. For the vector potential, we obtain :

$$\begin{bmatrix} A'_+ \\ A'_- \\ A'_0 \end{bmatrix}=A_0\begin{bmatrix} \frac{1}{2\sqrt{2}}\left(1+\frac{1}{\sqrt{3}}\right)e^{i(\mathbf{q}.\mathbf{r}-\omega t-\frac{\pi}{4})} - \frac{1}{2\sqrt{2}}\left(1-\frac{1}{\sqrt{3}}\right)e^{-i(\mathbf{q}.\mathbf{r}-\omega t-\frac{\pi}{4})} \\ \frac{1}{2\sqrt{2}}\left(1-\frac{1}{\sqrt{3}}\right)e^{i(\mathbf{q}.\mathbf{r}-\omega t-\frac{\pi}{4})} - \frac{e^{i\frac{\pi}{4}}}{2\sqrt{2}}\left(1+\frac{1}{\sqrt{3}}\right)e^{-i(\mathbf{q}.\mathbf{r}-\omega t-\frac{\pi}{4})} \\ -\frac{e^{i(\mathbf{q}.\mathbf{r}-\omega t-\frac{\pi}{4})}}{\sqrt{6}} \qquad -\frac{e^{-i(\mathbf{q}.\mathbf{r}-\omega t-\frac{\pi}{4})}}{\sqrt{6}} \end{bmatrix}$$

Which allows us to determine the vectors $\mathbf{A}_-(\mathbf{r},t)$ and $\mathbf{A}_+(\mathbf{r},t)=\mathbf{A}^*_-(\mathbf{r},t)$:

$$\mathbf{A}_-(\mathbf{r},t)=\frac{A_0}{\sqrt{2}}\left[+\frac{1}{2}\left(1+\frac{1}{\sqrt{3}}\right)\mathbf{e}'_+ + \frac{1}{2}\left(1-\frac{1}{\sqrt{3}}\right)\mathbf{e}'_- - \frac{1}{\sqrt{3}}\mathbf{e}'_0\right]e^{i(\mathbf{q}.\mathbf{r}-\omega t-\frac{\pi}{4})}$$

$$\mathbf{A}_+(\mathbf{r},t)=\frac{A_0}{\sqrt{2}}\left[-\frac{1}{2}\left(1-\frac{1}{\sqrt{3}}\right)\mathbf{e'}_+-\frac{1}{2}\left(1+\frac{1}{\sqrt{3}}\right)\mathbf{e'}_--\frac{1}{\sqrt{3}}\mathbf{e'}_0\right]e^{-i(\mathbf{q}.\mathbf{r}-\omega t-\frac{\pi}{4})}$$

Note that : $|\mathbf{A}_\pm(\mathbf{r},t)|=A_0/2$.

Finally, the optical Hamiltonian takes the form, in the basis $\mathcal{B}'_S$ :

$$\hat{H}_{opt}=\frac{e}{m_0c}\mathbf{A}(\mathbf{r},t).\hat{\mathbf{p}}=\frac{e}{m_0c}\left[\mathbf{A}_+(\mathbf{r},t).\hat{\mathbf{p}}+\mathbf{A}_-(\mathbf{r},t).\hat{\mathbf{p}}\right]$$

We define the two Fourier components $\hat{H}_\pm$ of the optical hamiltonian by:

$$\hat{H}_+(\mathbf{r},t)\equiv\frac{A_0}{\sqrt{2}}\left[\frac{1}{2}\left(1+\frac{1}{\sqrt{3}}\right)\hat{p}'_++\frac{1}{2}\left(1-\frac{1}{\sqrt{3}}\right)\hat{p}'_--\frac{1}{\sqrt{3}}\hat{p}'_0\right]e^{-i(\mathbf{q}.\mathbf{r}-\omega t-\frac{\pi}{4})}$$
$$\hat{H}_-(\mathbf{r},t)\equiv\frac{A_0}{\sqrt{2}}\left[-\frac{1}{2}\left(1-\frac{1}{\sqrt{3}}\right)\hat{p}'_+-\frac{1}{2}\left(1+\frac{1}{\sqrt{3}}\right)\hat{p}'_--\frac{1}{\sqrt{3}}\hat{p}'_0\right]e^{i(\mathbf{q}.\mathbf{r}-\omega t-\frac{\pi}{4})}$$

So that: $\hat{H}_{opt}=\hat{H}_++\hat{H}_-$ and, since $\hat{p}_\mp=\hat{p}_\pm^\dagger$ and $\hat{p}_0=\hat{p}_0^\dagger$, $\hat{H}_-=\left(\hat{H}_+\right)^\dagger$.

In order to specify the optical transitions at the $L_1$ point, the electronics valence and conductions states symmetry can be obtained for $C_{3v}$ point group using [2] as :

| Notation used in the core of the paper | Representation [1] | spin-orbital | angular momentum | band |
|---|---|---|---|---|
| $L_6$ | $L_4^c$ | $\alpha\lvert S'\uparrow\rangle+\beta\lvert Z'\uparrow\rangle$ | $\left\lvert\frac{1}{2},+\frac{1}{2}\right\rangle_c$ | conduction |
| | | $\alpha\lvert S'\downarrow\rangle-\beta\lvert Z'\downarrow\rangle$ | $\left\lvert\frac{1}{2},-\frac{1}{2}\right\rangle_c$ | |
| $L_{4,5}$ | $L_5^v+L_6^v$ | $-\left\lvert\frac{X'+iY'}{2}\uparrow\right\rangle$ | $\left\lvert\frac{3}{2},+\frac{3}{2}\right\rangle_v$ | heavy-valence |
| | | $\left\lvert\frac{X'-iY'}{2}\downarrow\right\rangle$ | $\left\lvert\frac{3}{2},-\frac{3}{2}\right\rangle_v$ | |
| $L_6$ | $L_4^v$ | $\left\lvert\frac{X'+iY'}{2}\downarrow\right\rangle$ | $\left\lvert\frac{1}{2},+\frac{1}{2}\right\rangle_v$ | spin-orbit valence |
| | | $\left\lvert\frac{X'-iY'}{2}\uparrow\right\rangle$ | $\left\lvert\frac{1}{2},-\frac{1}{2}\right\rangle_v$ | |

**Table S1**: The L-valley electronic states representation in $C_{3v}$

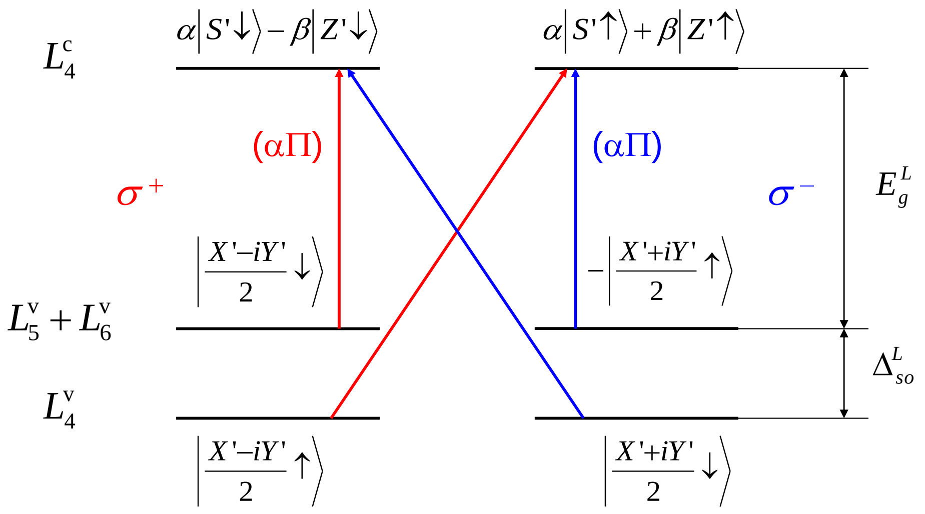


**Fig S1**: The optical transitions schele at L point in the GaAs Brillouin zone. The transition amplitudes ($\alpha\Pi$) represents $\langle u_c|\pm p_{\mp}|u_v\rangle$ matrix elements. For the notations, see text and table S1.

Note that the basis vectors of the sum of representation $L_5^v+L_6^v$ are eigenvectors of the hamiltonian since no longitudinal magnetic field is applied here. Here, we have defined the matrix element $\Pi\equiv\langle S'|\hat{p}'_x|X'\rangle=\langle S'|\hat{p}'_y|Y'\rangle$.
Using this notation, the coupling table with $\hat{p}'_\pm$ operators are easily obtained, and are summarised in the figure S1. The $\hat{p}'_0$ operator does not couple the mentioned conduction and valence states.

Now, we turn back to our excitation configuration with $\sigma^+$ photons propagating along [111]. The coupling table obtained from figure S1 is given in the following table S2.

| $\mathbf{e}.\hat{\mathbf{p}}$ <br> $\sigma^+$; $\mathbf{q}\parallel[1,1,1]$ | $\left\|\frac{X'-iY'}{2}\downarrow\right\rangle$ | $-\left\|\frac{X'+iY'}{2}\uparrow\right\rangle$ |
|---|---|---|
| $\alpha\|S'\downarrow\rangle-\beta\|Z'\downarrow\rangle$ | $-\frac{e^{-i\frac{\pi}{4}}}{2}\left(1+\frac{1}{\sqrt{3}}\right)\alpha\Pi$ | 0 |
| $\alpha\|S'\uparrow\rangle+\beta\|Z'\uparrow\rangle$ | 0 | $\frac{e^{-i\frac{\pi}{4}}}{2}\left(1-\frac{1}{\sqrt{3}}\right)\alpha\Pi$ |

**Table S2**: The coupling table for $\sigma^+$ photons propagating along [111] at L point.

A similar table can be obtained between the $L_4^v$ and $L_4^c$ band. From these tables (S1, S2) and figure S1, it can be inferred that no spin coherences can arise in the conduction band neither with a monochromatic, nor a 1 ps laser pulse. The spin polarization of the generated population is then deduced from (S15), which yields:

$$\mathbf{S}_c^{L_1}\Big|_{gen}=-\frac{\hbar}{2}\frac{\sqrt{3}}{2}\mathbf{e}'_z \qquad \text{(S18)}$$

For the opposite valley $\mathbf{e}''_z = -\mathbf{e}'_z$, oriented along [–1 –1 –1], it can be easily shown that the generated spin is :

$$\mathbf{S}_{\mathrm{c}}^{\mathrm{L}_1}\Big|_{gen} = +\frac{\hbar}{2}\frac{\sqrt{3}}{2}\mathbf{e}''_z \qquad \text{(S19)}$$

The spin generated in the other valleys is finally obtained using the invariance of the crystal by rotations around the $\mathbf{e}_z$ = [001] axis. Finally, the total average spin generated by a $\sigma^+$ polarised laser beam propagating along [001] is:

$$\mathbf{S}_{\mathrm{c}}\Big|_{gen} = \frac{1}{8}\sum_{i=1}^{8}\mathbf{S}_{\mathrm{c}}^{\mathrm{L}_i}\Big|_{gen} = -\frac{\hbar}{2}\frac{\mathbf{e}_z}{2} \qquad \text{(S20)}$$

Using the notation of the paper, this correspond to an absolute value photogenerated spin polarization $P_0^L = 50\%$. This initial spin will then decay equally in each L valleys, with no spin coherence arising. It will be then transferred to the Γ valley.

**References :**


[1] A. Messiah, *Quantum Mechanics*, Dover publications, 1999.

[2] G. F. Koster, J. O. Dimmock, G. Wheeler, R. G. Satz, Properties of thirty-two point groups (M.I.T. Press, Cambridge, Massachusetts USA) 1963.
